# Supplementary material for: Learning to Reason and Memorize with Self-Notes
Source: arXiv:2305.00833 source file (2023-10-31)
Supplement: Supplementary file 1 [file appendix1.tex]

\begin{table*}[ht]
    \caption{
    Test sample from the Algorithmic task. In this example, the question ($Q^*$) is ``\texttt{\textbf{print d}}'' and the answer ($A^*$) is ``\texttt{d = 3 ;}''. The vanilla model fails at tracking the variable(s) and incorrectly predicts ``\texttt{d = 2 ;}''. The scratchpad runs past the GPT-2 context length, since the context window also includes the input text, and thus cannot generate a valid scratchpad end token, so it can't make a prediction. The \selfnotes{} method correctly tracks the state of each variable as it sees statements, and successfully predicts ``\texttt{d = 3 ;}''.
    }
    
    \footnotesize
    \hskip-0.25cm\begin{tabular}{p{0.18\textwidth}|p{0.65\textwidth}|p{0.1\textwidth}}
    \hline
    \vspace{0.05pt}
     \textbf{\phantom{11111}Model}    &  
     \vspace{0.05pt}
\phantom{11111111111111111111111}\textbf{Context}     &  
    \vspace{0.001pt}
     \textbf{Prediction} \\\hline

     \vspace{0.5pt}\begin{tabular}[c]{@{}c@{}}Vanilla\\ (original context)\vspace{5pt}\end{tabular} & \vspace{0.5pt}\scriptsize{\texttt{d = 6 ; c = 10 ; a = 10 ; d ++ ; if d < 1 : b = 8 ; c -- ; d -- ; d -- ; a -- ; b = 7 ; b ++ ; e = 3 ; a -- ; b -- ; if d < 10 : b -- ; d -- ; if d < c : a ++ ; e -- ; b ++ ; a ++ ; if c > 3 : b ++ ; e -- ; if e > d : b ++ ; if a > 8 : e ++ ; b ++ ; if c < 7 : b -- ; c -- ; b ++ ; d ++ ; e ++ ; a -- ; if d < c : c ++ ; if e < 5 : b -- ; d -- ; if c > e : c ++ ; if b > 7 : b -- ; if d < b : d ++ ; c -- ; if c < d : e -- ; b -- ; c ++ ; d ++ ; e ++ ; b ++ ; d ++ ; b ++ ; e -- ; d -- ; if b < a : b ++ ; e -- ; if b < 9 : b -- ; a ++ ; if c > 10 : a -- ; b ++ ; c -- ; d ++ ; b -- ; b -- ; d ++ ; c ++ ; e -- ; if c > b : e ++ ; if c > b : d -- ; b ++ ; e -- ; c -- ; a -- ; if c > 1 : e ++ ; if e < d : c ++ ; if e < 1 : c -- ; a ++ ; d -- ; b -- ; c -- ; c -- ; if a > 4 : b -- ; b ++ ; d -- ; b ++ ; d -- ; e -- ; if a < 9 : e ++ ; if c < d : c -- ; a -- ; c ++ ; b -- ; if a > 8 : d ++ ; a -- ; d -- ; d -- ; c -- ; b ++ ; a -- ; c ++ ; \vspace{5pt}
}} & \vspace{0.5pt}\scriptsize{\texttt{d = 2 ;}} \\ \hline
 \vspace{0.5pt}\begin{tabular}[c]{@{}c@{}}Scratchpad\\ (scratchpad context)\vspace{5pt}\end{tabular} & \vspace{5pt}\scriptsize{\textrm{[invalid scratchpad generation]}} & \vspace{5pt}\scriptsize{ N/A }  \\\hline
\vspace{0.5pt}\begin{tabular}[c]{@{}c@{}}\selfnotes{}\vspace{5pt}\end{tabular} & \vspace{0.5pt}\scriptsize{\texttt{c = 10 ; print c  c = 10 ; a = 10 ; print a  a = 10 ; d ++ ; print d  d = 7 ; if d < 1 : b = 8 ; c -- ; print c  c = 9 ; d -- ; print d  d = 6 ; d -- ; print d  d = 5 ; a -- ; print a  a = 9 ; b = 7 ; print b  b = 7 ; b ++ ; print b  b = 8 ; e = 3 ; print e  e = 3 ; a -- ; print a  a = 8 ; b -- ; print b  b = 7 ; if d < 10 : b -- ; print b  b = 6 ; d -- ; print d  d = 4 ; if d < c : a ++ ; print a  a = 9 ; e -- ; print e  e = 2 ; b ++ ; print b  b = 7 ; a ++ ; print a  a = 10 ; if c > 3 : b ++ ; print b  b = 8 ; e -- ; print e  e = 1 ; if e > d : b ++ ; print b  b = 8 ; if a > 8 : e ++ ; print e  e = 2 ; b ++ ; print b  b = 9 ; if c < 7 : b -- ; print b  b = 9 ; c -- ; print c  c = 8 ; b ++ ; print b  b = 10 ; d ++ ; print d  d = 5 ; e ++ ; print e  e = 3 ; a -- ; print a  a = 9 ; if d < c : c ++ ; print c  c = 9 ; if e < 5 : b -- ; print b  b = 9 ; d -- ; print d  d = 4 ; if c > e : c ++ ; print c  c = 10 ; if b > 7 : b -- ; print b  b = 8 ; if d < b : d ++ ; print d  d = 5 ; c -- ; print c  c = 9 ; if c < d : e -- ; print e  e = 3 ; b -- ; print b  b = 7 ; c ++ ; print c  c = 10 ; d ++ ; print d  d = 6 ; e ++ ; print e  e = 4 ; b ++ ; print b  b = 8 ; d ++ ; print d  d = 7 ; b ++ ; print b  b = 9 ; e -- ; print e  e = 3 ; d -- ; print d  d = 6 ; if b < a : b ++ ; print b  b = 9 ; e -- ; print e  e = 2 ; if b < 9 : b -- ; print b  b = 9 ; a ++ ; print a  a = 10 ; if c > 10 : a -- ; print a  a = 10 ; b ++ ; print b  b = 10 ; c -- ; print c  c = 9 ; d ++ ; print d  d = 7 ; b -- ; print b  b = 9 ; b -- ; print b  b = 8 ; d ++ ; print d  d = 8 ; c ++ ; print c  c = 10 ; e -- ; print e  e = 1 ; if c > b : e ++ ; print e  e = 2 ; if c > b : d -- ; print d  d = 7 ; b ++ ; print b  b = 9 ; e -- ; print e  e = 1 ; c -- ; print c  c = 9 ; a -- ; print a  a = 9 ; if c > 1 : e ++ ; print e  e = 2 ; if e < d : c ++ ; print c  c = 10 ; if e < 1 : c -- ; print c  c = 10 ; a ++ ; print a  a = 10 ; d -- ; print d  d = 6 ; b -- ; print b  b = 8 ; c -- ; print c  c = 9 ; c -- ; print c  c = 8 ; if a > 4 : b -- ; print b  b = 7 ; b ++ ; print b  b = 8 ; d -- ; print d  d = 5 ; b ++ ; print b  b = 9 ; d -- ; print d  d = 4 ; e -- ; print e  e = 1 ; if a < 9 : e ++ ; print e  e = 1 ; if c < d : c -- ; print c  c = 8 ; a -- ; print a  a = 9 ; c ++ ; print c  c = 9 ; b -- ; print b  b = 8 ; if a > 8 : d ++ ; print d  d = 5 ; a -- ; print a  a = 8 ; d -- ; print d  d = 4 ; d -- ; print d  d = 3 ; c -- ; print c  c = 8 ; b ++ ; print b  b = 9 ; a -- ; print a  a = 7 ; c ++ ; print c  c = 9 ; \vspace{5pt}
}} & \vspace{0.5pt}\scriptsize{\texttt{d = 3 ;}}\\\hline
    \end{tabular}
    
    \label{tab:algo_sample}
\end{table*}
